# Supplementary material for: Flat bands in bilayer graphene induced by proximity with polar $h$-BN superlattices
Source: arXiv:2305.09749 ancillary file (2023-05-26)
Supplement: Supplementary file 1 [file supporting.pdf]

# Supporting Information for “Flat bands in bilayer graphene induced by proximity with polar *h*-BN superlattices”

Marta Brzezińska<sup>1</sup> and Oleg V. Yazyev<sup>1</sup>

<sup>1</sup>*Institute of Physics, Ecole Polytechnique Fédérale de Lausanne (EPFL), CH-1015 Lausanne, Switzerland*

## I. COMPUTATIONAL METHODOLOGY

DFT calculations were performed using the QUANTUM ESPRESSO suite<sup>1–3</sup> in conjunction with the Perdew-Burke-Ernzerhof (PBE)<sup>4,5</sup> exchange-correlation functional and norm-conserving pseudopotentials from PseudoDojo<sup>6</sup>. The vdW corrections are incorporated by employing the PBE+rvv10 method yielding excellent structural properties for layered materials<sup>7,8</sup> and find the interlayer distances  $d$  between C, B, and N atoms in relaxed structures to be close to the value in bulk graphite and BN<sup>9</sup>,  $d = 3.35$  Å. Data preprocessing was carried out with Atomic Simulator Environment (ASE)<sup>10</sup>. For the self-consistent calculations, we set the plane-waves basis cutoff to 80 Ry and used a fine Monkhorst-Pack  $\mathbf{k}$ -point grid of  $(90 \times 90 \times 1)$ . We verified that a vacuum region of thickness of 28 Å and 22 Å for  $2h$ -BN/BLG/ $2h$ -BN and  $2h$ -BN/BLG systems, respectively, is sufficient to avoid interactions between periodic images. Tight DFT convergence parameters were necessary to obtain consistent results for symmetry-related configurations. The Wannierization procedure was performed by employing the Wannier90 code<sup>11</sup>. The on-site matrix elements of an *ab initio* Hamiltonian were used to construct TB models within Pybinding package<sup>12</sup>. To solve a large-scale diagonalization problem, we used the FEAST algorithm<sup>13</sup>.

## II. EQUILIBRIUM INTERLAYER DISTANCE IN *h*-BN SYSTEMS

The vertical polarization  $P_z$  in layered materials was found to depend strongly on the interlayer distance  $d$ , and the optimal distance  $d_0$  considerably depends on how the vdW interactions are incorporated in the calculations. As (semi)-local functionals cannot correctly describe the long-range vdW interactions<sup>14</sup>, we systematically study various empirical correction schemes and non-local functionals in order to determine  $d_0$  (at fixed intralayer lattice constant  $a = 2.46$  Å) and the binding energies  $E_b$  of bulk and bilayer  $2h$ -BN systems in AB and AA' stacking configurations. We define the binding energy as

$$E_b = E_{2h\text{-BN}}(d_0) - E_{h\text{-BN}}, \quad (1)$$

where  $E_{2h\text{-BN}}$  is the energy of a two-layered system at optimal spacing  $d_0$ , and  $E_{h\text{-BN}}$  corresponds to the energy of a monolayer. As a reference system (monolayer), we use a supercell with two equally separated *h*-BN layers by a distance  $d = 16$  Å. We carried out calculations for the binding energies of bulk and bilayer geometries

using  $\mathbf{k}$ -point meshes of  $(27 \times 27 \times 9)$  and  $(27 \times 27 \times 1)$ , respectively. The results for dispersion-corrected LDA and PBE functionals<sup>15–21</sup> as well as for vdW functionals<sup>7,8,22–29</sup> are given in Table I.

The calculated values of  $d_0$  are in agreement with previous reports<sup>30–33</sup>. We recall that the experimentally determined interlayer distance in bulk *h*-BN (AA' configuration) is 3.33 Å<sup>34,35</sup>, which is closely reproduced by random phase approximation (RPA) calculations,  $d_0 = 3.34$  Å<sup>32</sup>. In general, the interlayer spacings  $d_0$  tend to be larger for AA' stacking order than AB; a similar trend is observed between bilayer and bulk geometries for the same stacking configurations.

We find that the binding energies are weaker in *h*-BN bilayers than in bulk systems. LDA functional in combination with DFT-D2 approach of Grimme (LDA-D2) yields overestimated values of  $E_b$ , while PBE is underbinding. We include these results solely for the purpose of conducting systematic investigations. The obtained binding energies using PBE+Grimme corrections and vdW-DFs functionals are consistent with Refs. 25, 32, and 33. However, our calculated binding energies using PBE-TS method are significantly lower than the values reported in previous articles<sup>30,33</sup>. We relate these differences to different computational setups employed between our study and other works. Ref. 36 reports interlayer binding energy from RPA calculations to be 39 meV/atom.

## III. POLARIZATION IN MULTILAYERED GRAPHENE/*h*-BN STRUCTURES

A commonly used approach to compute the polarization within the DFT framework deals with the Berry phase<sup>37,38</sup>. However, this method can be applied only to insulating systems. In this work, we estimate the vertical polarization  $P_z$  from the dipole corrections for a slab<sup>39–41</sup>. We summarize the results in Tables II and III. We indicate the stacking orders discussed in the main text by bold font. We stress that for symmetry-related  $2h$ -BN/BLG/ $2h$ -BN structures,  $P_z$  must be the same, but with opposite sign. A small discrepancy between these values up to 3% is due to numerical accuracy. For the sake of completeness, we also report the results for 8 stackings with inversion symmetry. As expected,  $P_z$  and  $\Delta E$  are practically zero.

It is important to stress that for *h*-BN bilayers (with large  $\Delta E$ ), the values of  $P_z$  obtained from dipole corrections and the Berry phase calculations with artificially

TABLE I. Equilibrium interlayer distance  $d_0$  and binding energy  $E_b$  for bulk and bilayer 2h-BN calculated using different dispersion corrections and non-local exchange-correlation functionals. All the binding energies are given in meV per atom in the four-atom unit cell.

|                  | bulk      |                     |           |                     | bilayer   |                     |           |                     |
|------------------|-----------|---------------------|-----------|---------------------|-----------|---------------------|-----------|---------------------|
|                  | AA'       |                     | AB        |                     | AA'       |                     | AB        |                     |
|                  | $d_0$ [Å] | $E_b$<br>[meV/atom] |
| LDA              | 3.22      | -26.8               | 3.22      | -27.7               | 3.25      | -13.4               | 3.22      | -13.9               |
| LDA-D2           | 2.91      | -143.0              | 2.88      | -148.7              | 2.94      | -65.9               | 2.89      | -69.0               |
| PBE              | 4.22      | -1.8                | 4.22      | -1.7                | 4.22      | -0.9                | 4.22      | -0.8                |
| PBE-D2           | 3.08      | -82.1               | 3.04      | -84.5               | 3.11      | -36.8               | 3.07      | -37.9               |
| PBE-D3           | 3.41      | -42.3               | 3.40      | -42.3               | 3.43      | -20.2               | 3.42      | -20.3               |
| PBE-D3<br>(BJ)   | 3.33      | -45.3               | 3.31      | -45.9               | 3.35      | -21.6               | 3.33      | -21.9               |
| PBE-D3M          | 3.27      | -41.9               | 3.25      | -42.6               | 3.29      | -20.1               | 3.26      | -20.4               |
| PBE-D3M<br>(BJ)  | 3.25      | -48.0               | 3.23      | -48.8               | 3.26      | -23.0               | 3.24      | -23.4               |
| PBE-TS           | 3.33      | -32.2               | 3.30      | -32.6               | 3.37      | -14.2               | 3.37      | -14.3               |
| PBE-MBD          | 3.45      | -23.7               | 3.45      | -23.9               | 3.44      | -11.0               | 3.44      | -11.1               |
| vdW-DF           | 3.55      | -53.3               | 3.53      | -53.2               | 3.57      | -24.0               | 3.56      | -23.9               |
| vdW-DF2          | 3.48      | -52.0               | 3.48      | -51.8               | 3.51      | -23.7               | 3.50      | -23.5               |
| vdW-DF-<br>C09   | 3.17      | -76.4               | 3.15      | -77.7               | 3.20      | -34.4               | 3.17      | -35.1               |
| vdW-DF2-<br>C09  | 3.22      | -55.2               | 3.20      | -55.3               | 3.25      | -24.4               | 3.23      | -24.8               |
| rev-vdW-<br>DF2  | 3.27      | -59.2               | 3.25      | -59.9               | 3.30      | -26.6               | 3.28      | -26.9               |
| vdW-DF-cx        | 3.22      | -65.5               | 3.20      | -66.6               | 3.25      | -29.2               | 3.23      | -29.6               |
| optB88-vdW       | 3.29      | -70.5               | 3.28      | -70.9               | 3.31      | -31.9               | 3.30      | -32.1               |
| optB86b-<br>vdW  | 3.25      | -70.7               | 3.24      | -71.4               | 3.28      | -31.9               | 3.26      | -32.2               |
| vdW-DF3-<br>opt1 | 3.25      | -56.0               | 3.23      | -56.7               | 3.26      | -25.9               | 3.25      | -26.3               |
| vdW-DF3-<br>opt2 | 3.24      | -61.2               | 3.22      | -62.0               | 3.27      | -28.0               | 3.25      | -28.3               |
| rVV10            | 3.30      | -69.8               | 3.29      | -70.4               | 3.35      | -30.1               | 3.34      | -30.3               |

TABLE II. Vertical polarizations per area  $P_z/A$  and energy gaps  $\Delta E$  of 2h-BN/BLG heterostructures.

| stacking    | $P_z/A$ [pC/m] | $\Delta E$ [meV] |
|-------------|----------------|------------------|
| ABAB        | 0.125          | 15.65            |
| ABAC        | 0.296          | 39.90            |
| ABCA        | -1.711         | 10.43            |
| ABCB        | -1.311         | 21.13            |
| ACAB        | 0.564          | 3.31             |
| ACAC        | 0.948          | 26.96            |
| <b>ACBA</b> | <b>2.555</b>   | <b>46.42</b>     |
| ACBC        | 2.386          | 21.45            |

introduced  $k$ -point sampling along  $z$ -axis are essentially the same. However, for graphene/ $h$ -BN structures char-

acterized by small  $\Delta E$ , the values of  $P_z$  obtained from the Berry phase calculations is more sensitive to the computational parameters.

#### IV. WANNIER FUNCTIONS ANALYSIS

To ensure the high quality of the Wannier functions and the convergence of the on-site energies, we performed wannierization on the  $30 \times 30 \times 1$   $\mathbf{k}$ -point meshes and chose the frozen window such that its edges are 1 meV away from the closest bands outside of the window. The resulting Wannier functions are atomic-like, with a total spread below 7 Å<sup>2</sup>. In Tables IV and V, we list the potential differences  $\Delta V_{\text{sublattice,U/L}}$  and  $\Delta_{\text{layer}}$  for all configurations considered.

TABLE III. Vertical polarization per area  $P_z/A$  and energy gap  $\Delta E$  calculated for  $2h$ -BN/BLG/ $2h$ -BN heterostructures in various stacking configurations.

| stacking | $P_z/A$ [pC/m] | $\Delta E$ [meV] | stacking      | $P_z/A$ [pC/m] | $\Delta E$ [meV] |
|----------|----------------|------------------|---------------|----------------|------------------|
| ABABAB   | -0.939         | 5.12             | ABABAC        | 1.483          | 7.14             |
| ACACAC   | 0.936          | 5.02             | ABCBCB        | -1.494         | 7.01             |
| ABABCA   | -2.583         | 23.42            | ABABCB        | -0.270         | 18.56            |
| ACBABA   | 2.589          | 23.38            | ABACAC        | 0.273          | 18.35            |
| ABACAB   | -2.062         | 14.47            | ABACBA        | 1.977          | 57.43            |
| ACBCAC   | 2.064          | 14.66            | ABCABA        | -1.982         | 57.44            |
| ABACBC   | -0.364         | 51.74            | <b>ABCABC</b> | <b>-4.296</b>  | <b>62.35</b>     |
| ACABCB   | 0.355          | 52.20            | ACBACB        | 4.296          | 61.84            |
| ABCACA   | -2.659         | 42.96            | ABCACB        | -0.341         | 38.88            |
| ACACBA   | 2.641          | 43.14            | ABCBAC        | 0.335          | 38.52            |
| ABCBAB   | -2.020         | 34.08            | ABCBCA        | -3.808         | 3.15             |
| ACABAC   | 2.013          | 34.00            | ACBCBA        | 3.804          | 3.31             |
| ACABAB   | -0.331         | 37.78            | ACABCA        | -1.955         | 57.61            |
| ACACBC   | 0.330          | 37.83            | ACBACA        | 1.970          | 56.88            |
| ACACAB   | -1.482         | 6.95             | ACBABC        | 0.283          | 19.06            |
| ACBCBC   | 1.475          | 7.19             | ACBCAB        | -0.274         | 19.26            |
| ABABA'C' | -2.319         | 3.96             | ABCBC'B'      | -2.326         | 2.34             |
| ACBCB'C' | 2.320          | 4.01             | ACACA'B'      | 2.327          | 2.24             |
| ABABC'A' | 1.792          | 31.94            | ACBAB'A'      | 1.724          | 10.84            |
| ABCAC'A' | -1.802         | 31.91            | ACACB'A'      | -1.725         | 11.00            |
| ABABC'B' | -0.536         | 26.83            | ABACA'C'      | -0.593         | 5.71             |
| ACABA'B' | 0.537          | 26.60            | ACACBC        | 0.587          | 5.65             |
| ABACA'B' | 1.732          | 9.99             | ACBCA'C'      | 1.777          | 31.25            |
| ABCBA'B' | -1.738         | 10.04            | ACABA'C'      | -1.786         | 31.08            |
| ABACB'A' | -2.328         | 3.79             | ABCAB'A'      | -2.428         | < 1              |
| ACBAC'A' | 2.325          | 3.78             | ACABC'A'      | 2.422          | < 1              |
| ABCAC'B' | -4.109         | 36.02            | ABCBA'C'      | -4.069         | 14.10            |
| ACBCA'B' | 4.110          | 35.89            | ACBAB'C'      | 4.054          | 14.29            |
| ABABA'B' | -0.001         | < 1              | ACACA'C'      | -0.004         | < 1              |
| ABACB'C' | -0.002         | < 1              | ACABC'B'      | -0.002         | < 1              |
| ABCAB'C' | -0.005         | < 1              | ACBAC'B'      | 0.003          | < 1              |
| ABCBC'A' | -0.007         | < 1              | ACBCB'A'      | 0.003          | < 1              |

## V. REAL-SPACE LOCALIZATION OF THE FLAT-BAND STATES

In Fig. 1, we show the sum of probability densities of two-fold degenerate eigenstates  $\psi_i$  at the  $\Gamma$  point,  $|\psi_i(\mathbf{r}, \mathbf{k} = 0)|^2$  at  $L = 50$  nm. These states are mostly localized in the centers or the corners of triangular domains, rather than at their edges.

## VI. BAND STRUCTURES OF PRIMED CONFIGURATIONS

We now comment on the band structures corresponding to the configurations that break inversion symmetry only weakly. The results are qualitatively different from

those for non-primed stacking configurations as these systems at large  $L$  remain gapless and no separated flat bands are observed (see Fig. 2), despite comparable values of the potential differences. This underlines the importance of local atomic environment on the electronic properties in the discussed structures.

TABLE IV. On-site energy differences of the  $p_z$  orbitals of C atoms in  $2h$ -BN/BLG heterostructures.

| stacking    | $\Delta V_{\text{sublattice,U}}$<br>[meV] | $\Delta V_{\text{sublattice,L}}$<br>[meV] | $\Delta_{\text{layer}}$ [meV] |
|-------------|-------------------------------------------|-------------------------------------------|-------------------------------|
| ABAB        | -1.53                                     | 11.84                                     | 10.82                         |
| ABAC        | -0.37                                     | -8.81                                     | 21.74                         |
| ABCA        | -1.04                                     | 43.26                                     | -4.34                         |
| ABCB        | 0.60                                      | -40.27                                    | 21.46                         |
| ACAB        | -1.21                                     | 43.97                                     | -16.64                        |
| ACAC        | 0.56                                      | -41.07                                    | 10.63                         |
| <b>ACBA</b> | <b>0.14</b>                               | <b>-7.72</b>                              | <b>14.95</b>                  |
| ACBC        | -0.80                                     | 9.33                                      | 4.43                          |

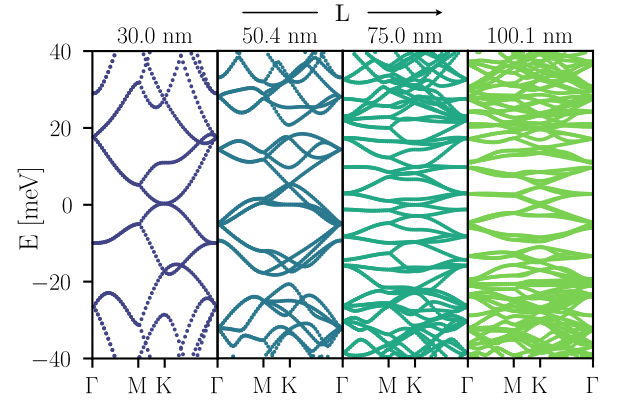

FIG. 2. Band structures as a function of  $L$  for the ABCAB'C' configuration. At  $L = 30$  nm, the parabolic band touching at  $K$  is present, which further evolves into a linear crossing.

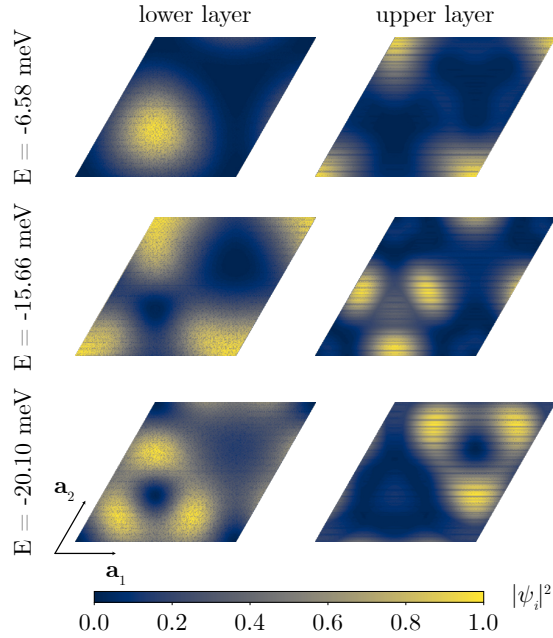

FIG. 1. Electronic density  $|\psi_i(\mathbf{r})|^2$  of the states from the marked flat bands subspaces (consult Fig. 2(c) of the main text). The color scale corresponds to the normalized square modulus  $|\psi_i(\mathbf{r})|^2$  of the wave function. The localization pattern exhibits a  $C_3$ -rotational symmetry.

TABLE V. On-site energy differences of the  $p_z$  orbitals of C atoms in  $2h$ -BN/BLG/ $2h$ -BN heterostructures.

| stacking | $\Delta V_{\text{sublattice,U}}$<br>[meV] | $\Delta V_{\text{sublattice,L}}$<br>[meV] | $\Delta_{\text{layer}}$ [meV] | stacking      | $\Delta V_{\text{sublattice,U}}$<br>[meV] | $\Delta V_{\text{sublattice,L}}$<br>[meV] | $\Delta_{\text{layer}}$ [meV] |
|----------|-------------------------------------------|-------------------------------------------|-------------------------------|---------------|-------------------------------------------|-------------------------------------------|-------------------------------|
| ABABAB   | 36.89                                     | 6.09                                      | -3.13                         | ABABAC        | 36.4                                      | 6.23                                      | -1.01                         |
| ACACAC   | -6.11                                     | -36.94                                    | 3.25                          | ABCBCB        | -6.25                                     | -36.43                                    | 1.17                          |
| ABABCA   | 5.03                                      | 7.42                                      | -13.47                        | ABABCB        | 5.88                                      | 7.26                                      | -17.00                        |
| ACBABA   | -7.41                                     | -5.08                                     | 13.53                         | ABACAC        | -7.34                                     | -5.89                                     | 17.28                         |
| ABACAB   | -6.69                                     | -5.80                                     | 20.13                         | ABACBA        | -37.08                                    | -4.98                                     | 31.83                         |
| ACBCAC   | 5.78                                      | 6.65                                      | -19.90                        | ABCABA        | 4.95                                      | 37.06                                     | -31.81                        |
| ABACBC   | -37.51                                    | -5.34                                     | 38.47                         | <b>ABCABC</b> | <b>4.70</b>                               | <b>36.09</b>                              | <b>-32.45</b>                 |
| ACABCB   | 5.32                                      | 37.45                                     | -37.91                        | ACBACB        | -36.09                                    | -4.74                                     | 33.06                         |
| ABCACA   | 36.42                                     | 36.28                                     | -19.91                        | ABCACB        | 36.63                                     | 37.16                                     | -23.94                        |
| ACACBA   | -36.31                                    | -36.46                                    | 19.72                         | ABCBAC        | -37.19                                    | -36.67                                    | 24.33                         |
| ABCBAB   | -37.10                                    | -35.85                                    | 27.10                         | ABCBCA        | -6.00                                     | -35.28                                    | 0.47                          |
| ACABAC   | 35.81                                     | 37.07                                     | -27.17                        | ACBCBA        | 35.2                                      | 5.97                                      | -0.24                         |
| ACABAB   | 35.96                                     | 37.54                                     | -23.95                        | ACABCA        | 4.61                                      | 37.57                                     | -37.31                        |
| ACACBC   | -37.58                                    | -36.01                                    | 23.94                         | ACBACA        | -37.57                                    | -4.66                                     | 38.14                         |
| ACACAB   | -5.76                                     | -36.47                                    | -3.51                         | ACBABC        | -6.22                                     | -6.64                                     | 17.98                         |
| ACBCBC   | 36.43                                     | 5.74                                      | 3.79                          | ACBCAB        | 6.64                                      | 6.19                                      | -17.75                        |
| ABABA'C' | -6.19                                     | 7.46                                      | 3.56                          | ABCBC'B'      | 37.25                                     | -36.62                                    | 4.04                          |
| ACBCB'C' | -7.49                                     | 6.18                                      | -3.59                         | ACACA'B'      | 36.60                                     | -37.28                                    | -3.90                         |
| ABABC'A' | -36.73                                    | 7.30                                      | 21.74                         | ACBAB'A'      | 35.40                                     | -5.57                                     | 20.71                         |
| ABCAC'A' | -7.29                                     | 36.70                                     | -21.76                        | ACACB'A'      | 5.57                                      | -35.46                                    | -20.49                        |
| ABABC'B' | -37.88                                    | 7.38                                      | 26.01                         | ABACA'C'      | 37.31                                     | -6.12                                     | 19.51                         |
| ACABA'B' | -7.39                                     | 37.82                                     | -26.23                        | ACACB'C'      | 6.10                                      | -37.36                                    | -19.52                        |
| ABACA'B' | 36.47                                     | -6.09                                     | 14.90                         | ACBCA'C'      | -37.71                                    | 7.76                                      | 25.24                         |
| ABCBA'B' | 6.07                                      | -36.49                                    | -14.81                        | ACABA'C'      | -7.78                                     | 37.70                                     | -25.42                        |
| ABACB'A' | 5.46                                      | -6.74                                     | 3.09                          | ABCAB'A'      | -38.16                                    | 36.95                                     | -2.22                         |
| ACBAC'A' | 6.73                                      | -5.46                                     | -3.06                         | ACABC'A'      | -37.02                                    | 38.09                                     | 1.60                          |
| ABCAC'B' | -7.06                                     | 35.73                                     | -21.65                        | ABCBA'C'      | 5.61                                      | -35.32                                    | -16.27                        |
| ACBCA'B' | -35.77                                    | 7.01                                      | 21.80                         | ACBAB'C'      | 35.27                                     | -5.68                                     | 16.11                         |
| ABABA'B' | -7.40                                     | 7.37                                      | 0.05                          | ACACA'C'      | 36.98                                     | -37.02                                    | -0.02                         |
| ABACB'C' | 6.24                                      | -6.28                                     | 0.04                          | ACABC'B'      | -37.82                                    | 37.80                                     | 0.06                          |
| ABCAB'C' | -38.05                                    | 38.02                                     | 0.07                          | ACBAC'B'      | 6.56                                      | -6.60                                     | 0.08                          |
| ABCBC'A' | 37.45                                     | -37.49                                    | 0.02                          | ACBCB'A'      | -5.55                                     | 5.52                                      | 0.07                          |

- <sup>1</sup> P. Giannozzi, S. Baroni, N. Bonini, M. Calandra, R. Car, C. Cavazzoni, D. Ceresoli, G. L. Chiarotti, M. Cococcioni, I. Dabo, A. D. Corso, S. de Gironcoli, S. Fabris, G. Fratesi, R. Gebauer, U. Gerstmann, C. Gougoussis, A. Kokalj, M. Lazzeri, L. Martin-Samos, N. Marzari, F. Mauri, R. Mazzarello, S. Paolini, A. Pasquarello, L. Paulatto, C. Sbraccia, S. Scandolo, G. Sclauzero, A. P. Seitsonen, A. Smogunov, P. Umari, and R. M. Wentzcovitch, *Journal of Physics: Condensed Matter* **21**, 395502 (2009).
- <sup>2</sup> P. Giannozzi, O. Andreussi, T. Brumme, O. Bunau, M. B. Nardelli, M. Calandra, R. Car, C. Cavazzoni, D. Ceresoli, M. Cococcioni, N. Colonna, I. Carnimeo, A. D. Corso, S. de Gironcoli, P. Delugas, R. A. DiStasio, A. Ferretti, A. Floris, G. Fratesi, G. Fugallo, R. Gebauer, U. Gerstmann, F. Giustino, T. Gorni, J. Jia, M. Kawamura, H.-Y. Ko, A. Kokalj, E. Küçükbenli, M. Lazzeri, M. Marsili, N. Marzari, F. Mauri, N. L. Nguyen, H.-V. Nguyen, A. O. de-la Roza, L. Paulatto, S. Poncé, D. Rocca, R. Sabatini, B. Santra, M. Schlipf, A. P. Seitsonen, A. Smogunov, I. Timrov, T. Thonhauser, P. Umari, N. Vast, X. Wu, and S. Baroni, *Journal of Physics: Condensed Matter* **29**, 465901 (2017).
- <sup>3</sup> P. Giannozzi, O. Baseggio, P. Bonfà, D. Brunato, R. Car, I. Carnimeo, C. Cavazzoni, S. de Gironcoli, P. Delugas, F. Ferrari Ruffino, A. Ferretti, N. Marzari, I. Timrov, A. Urru, and S. Baroni, *The Journal of Chemical Physics* **152**, 154105 (2020).
- <sup>4</sup> J. P. Perdew, K. Burke, and M. Ernzerhof, *Phys. Rev. Lett.* **77**, 3865 (1996).
- <sup>5</sup> J. P. Perdew, K. Burke, and M. Ernzerhof, *Phys. Rev. Lett.* **78**, 1396 (1997).
- <sup>6</sup> M. van Setten, M. Giantomassi, E. Bousquet, M. Verstraete, D. Hamann, X. Gonze, and G.-M. Rignanese, *Computer Physics Communications* **226**, 39 (2018).
- <sup>7</sup> R. Sabatini, T. Gorni, and S. de Gironcoli, *Phys. Rev. B* **87**, 041108 (2013).
- <sup>8</sup> H. Peng and J. P. Perdew, *Phys. Rev. B* **95**, 081105 (2017).
- <sup>9</sup> O. Hod, *Journal of Chemical Theory and Computation* **8**, 1360 (2012).
- <sup>10</sup> A. H. Larsen, J. J. Mortensen, J. Blomqvist, I. E. Castelli, R. Christensen, M. Dulak, J. Friis, M. N. Groves, B. Hammer, C. Hargus, E. D. Hermes, P. C. Jennings, P. B. Jensen, J. Kermode, J. R. Kitchin, E. L. Kolsbjerg, J. Kubal, K. Kaasbjerg, S. Lysgaard, J. B. Maronsson, T. Maxson, T. Olsen, L. Pastewka, A. Peterson, C. Rostgaard, J. Schiøtz, O. Schütt, M. Strange, K. S. Thygesen, T. Vegge, L. Vilhelmsen, M. Walter, Z. Zeng, and K. W. Jacobsen, *Journal of Physics: Condensed Matter* **29**, 273002 (2017).
- <sup>11</sup> A. A. Mostofi, J. R. Yates, G. Pizzi, Y.-S. Lee, I. Souza, D. Vanderbilt, and N. Marzari, *Computer Physics Communications* **185**, 2309 (2014).
- <sup>12</sup> D. Moldovan, M. Andelković, and F. Peeters, “pybinding v0.9.5: a python package for tight-binding calculations,” (2020).
- <sup>13</sup> E. Polizzi, *Phys. Rev. B* **79**, 115112 (2009).
- <sup>14</sup> Q. Wu and W. Yang, *The Journal of Chemical Physics* **116**, 515 (2002).
- <sup>15</sup> S. Grimme, *Journal of Computational Chemistry* **27**, 1787 (2006).
- <sup>16</sup> V. Barone, M. Casarin, D. Forrer, M. Pavone, M. Sambri, and A. Vittadini, *Journal of Computational Chemistry* **30**, 934 (2009).
- <sup>17</sup> S. Grimme, J. Antony, S. Ehrlich, and H. Krieg, *The Journal of Chemical Physics* **132**, 154104 (2010).
- <sup>18</sup> A. Tkatchenko and M. Scheffler, *Phys. Rev. Lett.* **102**, 073005 (2009).
- <sup>19</sup> A. Ambrosetti, A. M. Reilly, R. A. DiStasio, and A. Tkatchenko, *The Journal of Chemical Physics* **140**, 18A508 (2014).
- <sup>20</sup> A. D. Becke and E. R. Johnson, *The Journal of Chemical Physics* **127**, 154108 (2007).
- <sup>21</sup> A. Otero-de-la Roza and E. R. Johnson, *The Journal of Chemical Physics* **136**, 174109 (2012).
- <sup>22</sup> M. Dion, H. Rydberg, E. Schröder, D. C. Langreth, and B. I. Lundqvist, *Phys. Rev. Lett.* **92**, 246401 (2004).
- <sup>23</sup> T. Thonhauser, S. Zuluaga, C. A. Arter, K. Berland, E. Schröder, and P. Hyldgaard, *Phys. Rev. Lett.* **115**, 136402 (2015).
- <sup>24</sup> K. Lee, E. D. Murray, L. Kong, B. I. Lundqvist, and D. C. Langreth, *Phys. Rev. B* **82**, 081101 (2010).
- <sup>25</sup> I. Hamada, *Phys. Rev. B* **89**, 121103 (2014).
- <sup>26</sup> K. Berland and P. Hyldgaard, *Phys. Rev. B* **89**, 035412 (2014).
- <sup>27</sup> J. Klimeš, D. R. Bowler, and A. Michaelides, *Journal of Physics: Condensed Matter* **22**, 022201 (2009).
- <sup>28</sup> J. Klimeš, D. R. Bowler, and A. Michaelides, *Phys. Rev. B* **83**, 195131 (2011).
- <sup>29</sup> D. Chakraborty, K. Berland, and T. Thonhauser, *Journal of Chemical Theory and Computation* **16**, 5893 (2020).
- <sup>30</sup> N. Marom, J. Bernstein, J. Garel, A. Tkatchenko, E. Joselevich, L. Kronik, and O. Hod, *Phys. Rev. Lett.* **105**, 046801 (2010).
- <sup>31</sup> C.-R. Hsing, C. Cheng, J.-P. Chou, C.-M. Chang, and C.-M. Wei, *New Journal of Physics* **16**, 113015 (2014).
- <sup>32</sup> S. Zhou, J. Han, S. Dai, J. Sun, and D. J. Srolovitz, *Phys. Rev. B* **92**, 155438 (2015).
- <sup>33</sup> I. V. Lebedeva, A. V. Lebedev, A. M. Popov, and A. A. Knizhnik, *Computational Materials Science* **128**, 45 (2017).
- <sup>34</sup> R. S. Pease, *Nature* **165**, 722 (1950).
- <sup>35</sup> S. J. Haigh, A. Gholinia, R. Jalil, S. Romani, L. Britnell, D. C. Elias, K. S. Novoselov, L. A. Ponomarenko, A. K. Geim, and R. Gorbachev, *Nature Materials* **11**, 764 (2012).
- <sup>36</sup> T. Björkman, A. Gulans, A. V. Krasheninnikov, and R. M. Nieminen, *Journal of Physics: Condensed Matter* **24**, 424218 (2012).
- <sup>37</sup> R. Resta, *Ferroelectrics* **136**, 51 (1992).
- <sup>38</sup> D. Vanderbilt, *Berry Phases in Electronic Structure Theory: Electric Polarization, Orbital Magnetization and Topological Insulators* (Cambridge University Press, 2018).
- <sup>39</sup> R. Ramprasad and N. Shi, *Phys. Rev. B* **72**, 052107 (2005).
- <sup>40</sup> N. Shi and R. Ramprasad, *Applied Physics Letters* **91** (2007).
- <sup>41</sup> P. Strak, P. Kempisty, K. Sakowski, A. Kaminska, D. Jankowski, K. P. Korona, K. Sobczak, J. Borysiuk, M. Beeler, E. Grzanka, E. Monroy, and S. Krukowski, *AIP Advances* **7** (2017).
